# Supplementary material for: A Rademacher Complexity Based Method fo rControlling Power and Confidence Level in Adaptive Statistical Analysis
Source: arXiv:1910.03493 source file (2019-10-04)
Supplement: Supplementary file 1 [file appendix.tex]

\clearpage

\section{Two step application of the Martingale Central Limit Theorem:} It is possible to break the result in Theorem~\ref{thm:mclrad} into two parts: (1) a bound on the the generalization error $\Prob{\Psi (\mathcal{F}_k,\bar{x})-\Exp{\Psi (\mathcal{F}_k,\bar{x})}>\epsilon}$, and (2) a bound on the tightness of the proposed approximation of the Rademacher Complexity, that is $\Prob{R^{\mathcal{ F}_k}_{m}- \tilde{R}^{\mathcal{F}_k}_{\bar{x},\ell}>\epsilon}$. 

\begin{lemma}\label{lem:mcltgen}
\begin{equation*}
\lim_{m\rightarrow\infty} \Prob{\Psi (\mathcal{F}_k,\bar{x})-\Exp{\Psi (\mathcal{F}_k,\bar{x})}>\frac{\epsilon}{2\sqrt{m}}}\leq 1-\Phi(\epsilon).
\end{equation*}
\end{lemma}
\begin{proof}
Let us consider the Doob martingale for the function $\maxErr{\mathcal{F}_k,\bar{x}}$
\begin{equation}
C_i = \Exp{\maxErr{\mathcal{F}_k,\bar{x}}|X_1,\ldots,X_i}~~~i=0,\dots,m,
\end{equation}
which is defined with respect to the random variables $X_1,\ldots,X_m$, which correspond each to one of the elements in the sample $\bar{x}$. 
Let $Z_i = C_{i}-C_{i-1}$, for $1\leq i \leq m$, be the corresponding martingale difference sequence. 

In our setting $\forall x\in \mathcal{X}$ and $\forall f \in \mathcal{F}_k$, $f(x) \in [0,1]$, changing the value of any of the $m$ points in $\bar{x}$ can change $f(\bar{x})$ by at most $1/m$. Therefore, $|Z_i|\leq 1/m$, and $Z_i\in[\alpha,\beta]$ with $\beta - \alpha \leq 1/m$.
%Let:
%\begin{align}
%a_i &= (Z_{i+1}-Z_i|X_1,\ldots,X_i,f(X_i) = 0);\\
%b_i &= (Z_{i+1}-Z_i|X_1,\ldots,X_i,f(X_i) = 1);
%\end{align}
%Clearly, $a_i\Prob{a_i}+b_i\Prob{b_1} = 0 $. Hence, either $a_i=b_i = 0$, or at least one of the two values is negative. Assume without loss of generality that $b_i>a_i$, then $b_i-a_i \leq 1/m$. We have:
%\begin{align*}
%	&a_i\Prob{a_i}+b_i(1-\Prob{a_i}) = 0;\\
%	&a_i\Prob{a_i}+(\frac{1}{m}+a_i)(1-\Prob{a_i}) = 0.
%\end{align*}
%and thus:
%\begin{equation*}
%a_i = -\frac{1-\Prob{a_i}}{m}.
%\end{equation*}
%We can thus bound the value for $Z_i^2$:
%\begin{align*}
%Z_i^2 &\leq a_i^2\Prob{a_i}+b_i^2(1-\Prob{a_1})\\ &=  a_i\Prob{a_i}+(\frac{1}{m}+a_i)^2(1-\Prob{a_i})\\
%&\leq\frac{1}{m^2}\left((1-\Prob{a_i})^2\Prob{a_i}+(1-\Prob{a_i})\Prob{a_i}^2\right)\\
%&\leq \frac{1}{4m^2}.
%\end{align*}
%Where the last passage follows from the fact that $\left((1-\Prob{a_1})^2\Prob{a_i}+(1-\Prob{a_1})\Prob{a_i}^2\right)\leq 1/4$.
Given our definition of the difference martingale $Z_i$,  we have that for every $i$, $\Exp{Z_i}=0$, and hence, by applying Popoviciu's Inequality, we have:
\begin{equation*}
	\Exp{Z_i^2}=\Var{Z_i}\leq \frac{1}{4m^2}.
\end{equation*}
By linearity of expectation, $\sum_{i=1}^m Z_i = \Psi (\mathcal{F}_k,\bar{x})-\Exp{\Psi (\mathcal{F}_k,\bar{x})}$. Further, we have $\sum_{i=1}^m Z_i^2 \leq 1/4m$. By applying the MCLT we therefore have that $2\sqrt{m}\left(\Psi (\mathcal{F}_k,\bar{x})-\Exp{\Psi (\mathcal{F}_k,\bar{x})}\right)$ converges in distribution to $N(0,1)$ as $m$ goes to infinity. The lemma follows.
\end{proof}
 
We now show an application of the MCLT which allows to characterize the distribution of $R^{\mathcal{F}_k}_{m}- \tilde{R}^{\mathcal{F}_k}_{\bar{x}}$.

\begin{lemma}\label{lem:mcltrade}
\begin{equation}
\lim_{m\rightarrow\infty} \Prob{R^{\mathcal{F}_k}_{m}- \tilde{R}^{\mathcal{F}_k}_{\bar{x},\ell}>\frac{\sqrt{5}\epsilon}{2\sqrt{\ell m}}}\leq 1-\Phi(\epsilon).
 \end{equation}
\end{lemma}
\begin{proof}
The proof closely follows the steps of the proof of Theorem~\ref{lem:bernrade}.
In the following we assume $\ell \geq2$. Consider the Doob martingale $C_i$ and the martingale difference sequence $Z_i$ defined as in the proof of Theorem~\ref{lem:bernrade}.

% For the simplicity purposes, assume $Y_i = X_i$ for $1\leq i \leq m$, and the remaining $Y_i$ are the $\ell m$ independent Rademacher Random Variables which compose the $\ell$ vectors of Rademacher random variables. That is,  $Y_{j(m)+i}= \sigma_{j,i}$, for $1\leq j\leq \ell$ and $1\leq i \leq m$. By definition, $\tilde{R}_{\bar{x},\ell}^{\mathcal{F}_k}$ is a function of $m(\ell+1)$ independent random variables $Y_i$.
% Note that the sequence $Z_i$ defined here correspond to the martingale difference sequence by the same name which we studied in the proof of Theorem~\ref{lem:bernrade}. 

As shown in the proof of Theorem~\ref{lem:bernrade}, we have $\sum_{i=1}^{m(\ell+1)} Z_i^2 \leq 5/4\ell m$, and that $|Z_i|<1/m$ for all $1\leq i\leq m(\ell+1)$.
By linearity of expectation, $\sum_{i=1}^{\ell (m+1)} Z_i =  R^{\mathcal{F}_k}_{m}-\tilde{R}^{\mathcal{F}_k}_{\bar{x},\ell}$. 
%By applying the MCLT we therefore have:
%\begin{align*}
%&\lim_{m\rightarrow\infty} \Prob{\frac{2\sqrt{\ell m}}{\sqrt{5}}\left(\tilde{R}^{\mathcal F}_{\bar{x}} - R^{\mathcal F}_{\bar{x}}\right)>\epsilon}\\&\qquad\leq  \Prob{\tilde{R}^{\mathcal F}_{\bar{x}} - R^{\mathcal F}_{\bar{x}}> \frac{2\sqrt{\ell m}}{\sqrt{5}} \epsilon}\leq 1-\Phi(\frac{2\sqrt{\ell m}}{\sqrt{5}}\epsilon).
% \end{align*}

By applying the MCLT, we therefore have that $2\sqrt{\frac{\ell m}{5}}\left(R^{\mathcal{F}_k}_{m}-\tilde{R}^{\mathcal{F}_k}_{\bar{x},\ell}\right)$ converges in distribution to $N(0,1)$. The lemma follows. 
\end{proof}
% We can bound the generalization error in terms of the estimated \Rade{} of $\mathcal{F}_k$ as by combining the results of Theorem~\ref{th:Ra}, and Lemmas~\ref{lem:mcltgen}-~\ref{lem:mcltrade} using the union bound:
% \begin{theorem}
% \begin{equation}
% 	\lim_{m\rightarrow\infty} \Prob{\Psi (\mathcal{ F},\bar{x}) > 2\tilde{R}^{\cal F}_m+ \frac{\epsilon_1}{2\sqrt{m}}+\frac{\sqrt{5}\epsilon_2}{\sqrt{\ell m}}} \leq 2-\Phi(\epsilon_1)-\Phi(\epsilon_2).
% \end{equation}
% \end{theorem}
\section{Bounding the generalization error using McDiarmid's inequality}\label{app:refinedmcdia}

McDiarmid's inequality is a useful variation of the more general Azuma-Hoeffding inequality~\cite{mitzenmacher2017probability}.
% \begin{theorem}{Mc Diarmid's Inequality - Theorem 13.7~\cite{mitzenmacher2017probability}}
% Let $f$ be a function on $n$ variables that satisfies the Lipschitz condition with bound $c$. Let $X_1,\ldots,X_t$ be independent random variables each identically distributed according to the distribution $\mathcal{D}$, such that $f(X_1,\ldots,X_t)$ is in the domain of $f$. Then
% \begin{equation*}
% 	\Prob{\Expe{\mathcal{D}^t}{f(X_1,\ldots,X_t)}- f(X_1,\ldots,X_t) \geq \lambda}\leq e^{2\lambda^2}.
% \end{equation*}
% \end{theorem}
In the theory literature, McDiarmid's inequality is used to obtain bounds on both the generalization error (i.e., Theorem~\ref{th:Ra2}) and the difference between the \Rade{} and the Empirical \Rade{} for a given sample $\bar{x}$~\cite{ShalevSBD14}.An additional error is occurred in estimating the empirical Rademacher complexity using a finite number of Rademacher vectors.

Our proposed method eliminates this additional passage by estimating \emph{directly} the \Rade{} using as $\tilde{R}_{\bar{x},\ell}^{{\mathcal F}}$, computed according to equation~\eqref{eq:radestimate}.
% In this section we show that McDiarmid's inequality can be used to characterize the quality of the estimate of the the \Rade{}  of a given class $\mathcal{F}$ computed as $\tilde{R}_{\bar{x},\ell}^{{\mathcal F}}$ (equation~\eqref{eq:radestimate})

In~\cite{Barlett02} (Theorem 11), Bartlett et al. present a bound on the quality of the approximation of the \Rade{} achievable using a single vector of Rademacher random variables. Instead, the result presented here is a one-sided bound. Further, we achieve an improvement of the exponential term in the right-hand side of the bound by taking into considerations that the functions being considered are non-negative and  take values in $[0,1]$, and, crucially, by using multiple vectors of Rademacher random variables.

%Clearly $\Expe{\bar{x},\sigma_1,\dots,\sigma_\ell} {R_{\bar{x},\ell}^{{\mathcal F}}}=R^{{\cal F}}_m.$
\begin{lemma}\label{lem:mcdiarmid2}
	\begin{equation}\label{eq:mcdiarmid2}
		\Prob{R^{\mathcal{F}_k}_m - \tilde{R}_{\bar{x},\ell}^{\mathcal{F}_k}> \epsilon} \leq e^{-2m\ell\epsilon^2/\left(\ell+4\right)}.
	\end{equation}
\end{lemma}
\begin{proof}
Clearly $\tilde{R}_{\bar{x},\ell}^{{\mathcal F}_k}$ is a function of $m(\ell+1)$ independent Random variables $Y_i$. For the simplicity purposes, assume $Y_i = X_i$ for $1\leq i \leq m$, and the remaining $Y_i$ are the $\ell m$ independent Rademacher random variables which compose the $\ell$ vectors of Rademacher random variables.
		In order to apply McDiarmid's inequality we need to carefully bound the maximum  change of the the value of the function $\tilde{R}_{\bar{x},\ell}^{\mathcal{F}_k}$ when changing the the value of the $i$-th random variable $Y_i$, denoted as $c_i$.
\begin{itemize}
\item  $1\leq i \leq m$: as is our setting $\forall x\in \mathcal{X}$ and $\forall f \in \mathcal{F}_k$, $f(x) \in [0,1]$, changing the value of any of the $m$ points in $\bar{x}$ can change $f(\bar{x})$ by at most $1/m$. As we are considering the maximum deviation in expectation with respect to the value of the $m\ell$ Rademacher random variables we can conclude $c_i\leq 1/m$.
\item  $m+1\leq i\leq m (\ell+1)$: changing the value of one of the Rademacher random variables can change the value of $\tilde{R}_{\bar{x},\ell}^{\mathcal{F}_k}$ by at most  $\frac{2}{\ell m}$, hence, we have $c_i\leq \frac{2}{\ell m}$.
\end{itemize}
We therefore have:
$$\sum_{i=1}^{m(\ell+1)} c_i^2 = \sum_{i=1}^{m} c_i^2+ \sum_{i=m+1}^{m (\ell+1)} c_i^2 = \frac{1}{m}+ \frac{4}{\ell m} = \frac{\ell+4}{\ell m}.$$
The lemma follows by applying McDiarmid's inequality.
\end{proof}

Note that for high values of $\ell$, the right hand side of equation \eqref{eq:mcdiarmid2}, is close to $e^{-2km\epsilon^2}$. In a natural tradeoff, while using multiple vectors of Rademacher random variables does indeed allow to obtain a higher quality estimate of the \Rade{}, it also introduces a higher overhead time in the computation of the estimate.  

In order to improve both the time and memory space requirements of our algorithm, we can obtain an estimation of the \Rade{} $R^{\mathcal{F}_k}_m$ using a single vector of $m$ Rademacher random variables. In this case, we can obtain a slightly better guarantee on the accuracy of $\tilde{R}_{\bar{x},\ell}^{{\mathcal F}_k}$ than the one implied by~\eqref{eq:mcdiarmid2}:

\begin{lemma}\label{lem:mcdiarmid2v2}
\label{the:11}
$$\Prob{R^{\mathcal{ F}_k}_m >  \tilde{R}^{\mathcal{F}_k}_{\bar{x},1} + \epsilon} \leq e^{-m\epsilon^2/2}.$$
\end{lemma}

The proof of this lemma mostly follows the same steps as the one for Lemma~\ref{lem:mcdiarmid2}: the sharper bound is obtained by observing that $\tilde{R}_{\bar{x},1}^{\mathcal{F}_k}$ can be characterized as a function of just $m$ independent and identically distributed random variables $y_i = x_i\sigma_i$ from the product distribution $\mathcal{D}\times\sigma$.

Using the \emph{union bound} we can combine the results of  Theorem~\ref{th:Ra2} and Lemma~\ref{lem:mcdiarmid2} (or Lemma~\ref{lem:mcdiarmid2v2}) and obtain:
\begin{theorem}\label{eqn:es1}
	\begin{equation}
\Prob{\Psi (\mathcal{ F}_k,\bar{x}) > 2\tilde{R}^{\mathcal{F}_k}_m+ \epsilon_1+2\epsilon_2}\leq e^{-2m\epsilon_1^2}+e^{-2m\ell\epsilon^2/\left(\ell+4\right)}. 
\end{equation}
\end{theorem}
